# Supplementary material for: Experimental and Theoretical Investigation on the Possible Half-metallic Behaviour of Equiatomic Quaternary Heusler Alloys: CoRuMnGe and CoRuVZ (Z = Al, Ga)
Source: arXiv:1903.07265 source file (2019-08-02)
Supplement: Supplementary file 1 [file supplementary.pdf]

# Supplementary Information: Experimental and Theoretical Investigation on the Possible Half-metallic Behaviour of Equiatomic Quaternary Heusler Alloys: CoRuMnGe and CoRuVZ (Z = Al, Ga)

Deepika Rani[a], Lakhan Bainsla[a,b], K. G. Suresh[a] and Aftab Alam[a*]

[a] *Department of Physics, Indian Institute of Technology Bombay, Powai, Mumbai 400076, Maharashtra, India*

[b] *WPI Advanced Institute for Materials Research, Tohoku University, Sendai 980-8577, Japan*

(Dated: July 1, 2019)

## Abstract

Here, we provide supporting data for the effect of swap/antisite disorder on the magnetic properties of CoRuVAl.

Table S1. Magnetic moments ($\mu_B$) of ordered and swap disordered CoRuVAl in a ($2 \times 2 \times 2$) supercell. $X_d$ refers to defect atoms.

| System | Co1,2,3,4,5,6,7,8 | Ru1,2,3,4,5,6,7,8 | V1,2,3,4,5,6,7,8 | $X_d$ | $m_{total}(\mu_B/f.u.)$ |
|---|---|---|---|---|---|
| **Ordered** | 0.695 | -0.002 | 0.300 | | 0.96 |
| **Co-Ru swap** | 0.77, 0.76 | -0.03, -0.01 | 0.28, 0.29 | $Co_{Ru}$: 0.99 | 0.96 |
| (12.5 %) | 0.77, 0.77 | -0.02, 0.07 | 0.26, 0.29 | $Ru_{Co}$: -0.14 | |
| | 0.76, 0.29 | -0.01,-0.03 | 0.29, 0.27 | | |
| | 0.77, 0.99 | -0.14, -0.03 | 0.30, 0.28 | | |
| **V-Al swap** | 0.33, 0,33 | 0.04, 0.01 | 0.42, 0.45 | $V_{Al}$: 0.42 | 0.96 |
| (12.5 %) | 1.03, 1.04 | -0.01, -0.01 | 0.30, 0.30 | | |
| | 0.33, 1.03 | -0.02, 0.00 | 0.25, 0.28 | | |
| | 1.02, 0.30 | 0.01, -0.03 | 0.26, 0.29 | | |
| **Co-Ru and V-Al** | 1.069, 0.424 | -0.03, -0.03 | 0.61, 0.25 | $Co_{Ru}$: 0.84 | 0.97 |
| (12.5 %) | 0.948, 0.985 | -0.05, 0.02 | 0.25, 0.30 | $Ru_{Co}$: -0.05 | |
| | 0.422, 0.946 | -0.05,-0.04 | 0.27, 0.28 | $V_{Al}$: 0.31 | |
| | 0.644, 0.447 | -0.10, -0.06 | 0.27, 0.28 | | |

**Effect of disorder on Magnetic properties of CoRuVAl**

In case of CoRuVAl, the experimental magnetic moment is quite low (0.53 $\mu_B$/f.u.) as compared to the calculated moment (0.96 $\mu_B$/f.u.). In order to find the reason behind the experimentally observed low magnetic moment, the effect of disorder on its magnetic properties is studied in details. It has been observed by various researchers that swap or anti-site disorder has an important effect on the magnetic and electronic properties of Heusler alloys[1–4]. As from XRD, we expect disorder between Co and Ru sites as well as V and Al sites, we simulated different types of disorder between these sites and study their effect on the magnetic properties. We mainly focus on swap and anti-site type disorder in a $2 \times 2 \times 2$ supercell, which consists of 32 atoms, 8 of each type. In case of swap disorder, one atom is exchanged by other atom whereas, in case of anti-site disorder, one of the atom is replaced

Table S2.Magnetic moments ($\mu_B$) of anti-site disordered CoRuVAl in a $2 \times 2 \times 2$ supercell. $X_d$ refers to defect atoms.

| Antisite type | Co1,2,3,4,5,6,7,8 | Ru1,2,3,4,5,6,7,8 | V1,2,3,4,5,6,7,8 | $X_d$ | $m_{total}(\mu_B/f.u.)$ |
|---|---|---|---|---|---|
| **Type A** | | | | | |
| **Ru→Co** | 0.743, 0.735, | 0.061,-0.013, | 0.217, 0.309, | Ru: -0.104 | 0.80 |
| | 0.777, 0.128, | 0.000, -0.009, | 0.232, 0.287, | | |
| | 0.748, 0.754, | -0.010, -0.001, | 0.231, 0.281, | | |
| | 0.770, - | -0.008, 0.026 | 0.230, 0.287 | | |
| **Type B** | | | | | |
| **Al→V** | 0.312, 0.317, | -0.021,-0.028, | 0.243, 0.247, | Al: -0.006 | 0.72 |
| | 0.330, 0.314, | -0.018, -0.020, | 0.253, 0.251, | | |
| | 0.763, 0.739, | 0.015, 0.006, | 0.221, 0.231, | | |
| | 0.736, 0.741 | 0.003, 0.003 | 0.425, - | | |
| **Type C** | | | | | |
| **Ru→Co** and **Al→V** | 0.393, 0.382 | 0.018,-0.030 | 0.157, 0.219 | Ru: -0.088 | 0.57 |
| | 0.404, -0.028, | -0.012, -0.011, | 0.176, 0.224, | Al: -0.005 | |
| | 0.766, 0.753, | -0.003, 0.005, | 0.166, 0.211, | | |
| | 0.774, - | 0.004, 0.029 | 0.312, - | | |

by another atom.

Swap disorder

To simulate the swap disorder, a $2 \times 2 \times 2$ supercell of the primitive cell of the type I configuration of CRVA is constructed. All possible configurations for replacement of Co by Ru (V by Al) and vice versa was checked, and energetically the most stable configuration is chosen to present the result here. We have considered three types of swap disorder, 1) Co-Ru swap, 2) V-Al swap, and 3) Co-Ru and V-Al pairs swap. Exchanging one of the eight Co (V) atom positions and one of the eight Ru (Al) atom positions leads to 12.5 % swap disorder between Co(V) and Ru(Al) sites. Thus, B2-type structure is formed when 50%

swap disorders were simulated by exchanging four of the eight Co (V) atoms and four of the eight Ru (Al) atom positions. The local as well as the total moments for different types of swap disorder are tabulated in Table S1. Here Co1,2,3,4,5,6,7,8 represents the eight Co atoms in a $2\times2\times2$ supercell. By considering the swap disorder between Co & Ru sites and V & Al sites, we observed that the total magnetic moment remains almost the same as that of the ordered structure. This is due to the similar local environment of different atomic-sites in case of ordered and swap disordered structures. Even, the B2-type structure also gives the same magnetic moment as that of ordered structure. Thus, it is clear that swap disorder between these sites is not responsible for the lower magnetic moment. Another possibility is the anti-site disorder.

Anti-site disorder

We have also studied the effect of anti-site disorder between Co and Ru sites as well as V and Al sites. We have considered three types of anti-site disorder: 1) Type A (Ru$\rightarrow$Co), where one Co atom is replaced by Ru atom (which corresponds to 12.5 % anti-site disorder between Co and Ru sites), 2) Type B(Al$\rightarrow$V), where one V atom is replaced by Al atom and, 3) Type C (Ru$\rightarrow$Co and Al$\rightarrow$V), where one Co atom is replaced by Ru atom, and one V atom is replaced by Al atom, in a 32-atoms supercell. It is found that, the total magnetic moment are extremely sensitive to the anti-site disorder (antisite between Co & Ru and V & Al). Interestingly, due to the change in the local environment in this case, the local atomic moments change drastically; sometimes even get quenched and/or antiferromagnetically aligned as compared to the completely ordered case. The latter is attributed to the itinerant character of magnetism in Co, Ru, and V-containing Heusler alloys, and to the frustration of antiferromagnetic exchange interactions, accompanied by a tetragonal distortion. In fact, the exchange interaction in this case is reasonably long ranged, affecting the moment of atoms sitting far from the defected sites. Table S2 shows the simulated results for a 2x2x2 supercell which reduces the net cell moment up to 0.57 $\mu_B$, when antisite disorder between both (Co & Ru) and (V & Al) pairs are considered. The local moment at different sites also changes due to the different local environment in the disordered structure as compared to the ordered one. When both Co $\leftrightarrow$ Ru and V $\leftrightarrow$ Al type disorders are considered, the total moment nearly matches to the experimentally observed moment of 0.53 $\mu_B/f.u.$ A careful analysis shows that in this case, for Co1, Co2 and Co3 atoms the magnetic moment has decreased to almost half of the moment which Co possess in case of purely ordered

structure i.e. from 0.7 to 0.4 $\mu_B/f.u.$ In case of purely ordered structure, the Co atoms are surrounded by four V and four Al atoms. For Co1, Co2 and Co3 atoms, the nearest neighbors are three V and five Al atoms, however the bind lengths are slightly different for some of the sites (due to relaxation effect). In case of Co4-site, the atomic arrangement is similar to the above case i.e. Co atom is surrounded by 3 V and 5 Al atoms, however the bond lengths are different. In this case, the magnetic moment is reduced to a value of $\sim$ -0.03. In the case of Co5, Co6 and Co7, the Co-atoms have nearly the same magnetic moment as that of the purely ordered case. This is due to the similar local environment, as these sites are surrounded by 4 Al and 4 V atoms, similar to that of ordered structure. In case of purely ordered structure, the V atoms are surrounded by four Co and four Ru atoms. In the Type C disordered structure, 1V, 3V, 5V and 7V have three Co and five Ru atoms as their nearest neighbors, whereas 3V,4V and 6V are surrounded by four Al and four V atoms, similar to that of ordered structure. Thus, due to disorder, the nearest neighbors and bond lengths change, which in turn changes the local magnetic moment at the atomic sites and hence the total magnetic moment. We have also checked the effect of antisite disorder using a $3 \times 3 \times 3$ supercell (which is able to achieve a much lower swap concentration, 1/27 = 3.7 %), which yields a reduced moment up to 0.83 $\mu_B/f.u.$, when 3.7 % anti-site disorder between both (Co & Ru) and (V & Al) pairs are considered. Thus, we conclude that possibly the anti-site disorder between Co & Ru sites and V & Al sites is responsible for the low value of magnetic moment in case of CoRuVAl. Similar behavior has been observed in case of MnCrVAl, where the magnetic moment is quenched to zero because of disorder whereas, the ordered structure is expected to have a magnetic moment of 3 $\mu_B/f.u.$[1,2].

## REFERENCES

* aftab@phy.iitb.ac.in

1 J. Herran, R. Dalal, P. Gray, P. Kharel, and P. V. Lukashev, Journal of Applied Physics **122**, 153904 (2017).

2 P. Kharel, J. Herran, P. Lukashev, Y. Jin, J. Waybright, S. Gilbert, B. Staten, P. Gray, S. Valloppilly, Y. Huh, and D. J. Sellmyer, AIP Advances **7**, 056402 (2017).

[3] D. X. F. D. X. F. G. R. K. C. Z. X. W. L. Y. W. X. T. Lin, T. T and G. D. Liu, Scientific Reports **7**, 42034 (2017).

[4] Y. Feng, H. Chen, H. Yuan, Y. Zhou, and X. Chen, J. Magn. Magn. Mater. **378**, 7 (2015).
